# Supplementary material for: Optimal Circuit-Level Decoding for Surface Codes
Source: arXiv:1609.06373 ancillary file (2016-09-20)
Supplement: Supplementary file 1 [file supplemental_material.pdf]

# Supplemental Material for: Optimal Circuit-Level Decoding for Surface Codes

Bettina Heim,[1] Krysta M. Svore,[2] and Matthew B. Hastings[3,2]

[1] *Theoretische Physik, ETH Zurich, 8093 Zurich, Switzerland*
[2] *Station Q Quantum Architectures and Computation Group, Microsoft Research, Redmond, WA 98052, USA*
[3] *Station Q, Microsoft Research, Santa Barbara, CA 93106-6105, USA*

## SURFACE CODE LAYOUT AND SYNDROME EXTRACTION

The layout of the used surface code family for a distance $d = 5$ and $d = 6$ is shown in Fig.1. Black dots represent data qubits, red and blue dots represent ancilla qubits used to measure $X$- and $Z$- type stabilizer generators, respectively. The stabilizer generators consist of four $X$ ($Z$) operators acting on the four data qubits surrounding a red (blue) square. The circuits shown in Fig. 2 implement a projective measurement onto their eigenspaces. Excitations are reflected by a $-1$ measurement of the adjacent ancilla qubits, with $X$-type ($Z$-type) stabilizers detecting $Z$ ($X$) errors. An SN-circuit minimizes error propagation for both kinds of errors, whereas this is not the case for the CCC-circuit.

## DECODING ALGORITHMS

*Maximum Likelihood Decoding:* We will first discuss how to calculate the transition matrix for circuit level noise, describing transitions between EC-cosets. For a code with $n_a$ stabilizer generators encoding $k$ logical qubits, each EC-coset can be associated with a bitstring $r$, in which the first $n_a$ bits denote the ideal syndrome of all contained error patterns, the next $n_a$ bits the measured syndrome, and the final $2^k$ bits denote the logical correction needed for a full recovery from any of the contained error patterns. Consider an error pattern $E$

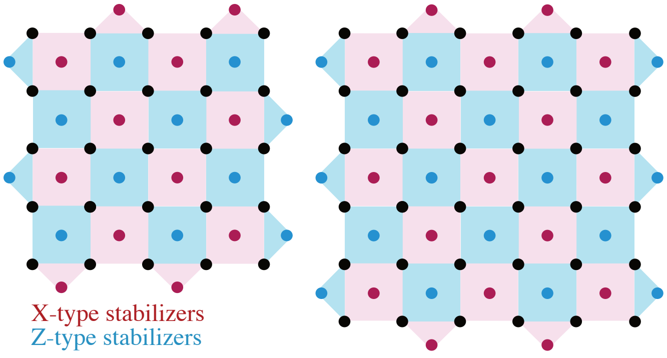


Figure 1. Layout of the used surface code family with a reduced number of physical qubits compared to commonly used surface codes. A distance $d$ code contains $d \times d$ data qubits, resulting in a total of $2d^2 - 1$ required (data and ancilla) qubits. On the left side is a distance five surface code with 49 qubits, denoted as Surface49 in the plots, on the right side is a distance six code with 71 qubits.

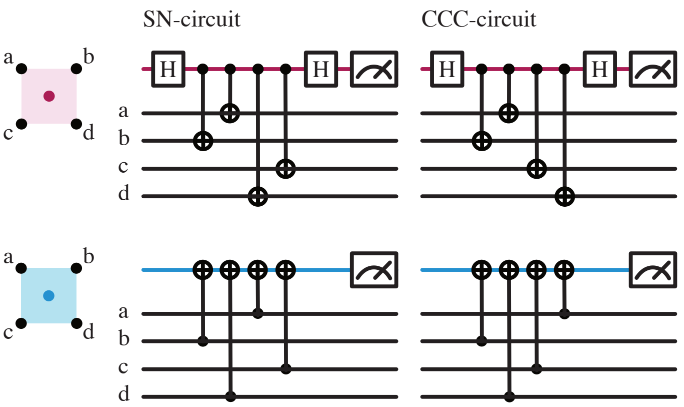


Figure 2. Measurement circuit for $X$- and $Z$-type stabilizers.

occurring with probability $p$ during the applied circuit ending in syndrome extraction, that contributes to a certain EC-coset characterized by a bitstring $r_E$ at the end of the circuit. The matrix elements of its transition matrix $T^E$ then are

$$t^E_{kl} = (1-p)\delta_{k,l} + p\delta_{k\,\hat{}\,l, r_E} \qquad (1)$$

where $\hat{}$ denotes the bitwise OR operation. This matrix is diagonal in Hadamard basis. Let $H$ be the Hadamard transformation on a vector space of dimension $4^{n_a+k} := N$, with matrix elements $h_{ik} = (-1)^{i*k}/\sqrt{N}$. Here, $*$ denotes the bitwise dot product of the binary representations of $i = \sum_q i_q 2^q$ and $k = \sum_q k_q 2^q$, that is $i * k = \sum_q i_q \,\&\, k_q$ for & the bitwise AND operation. Then

$$
\begin{aligned}
(HT^E H)_{ij} &= \sum_{k,l} h_{ik}\, t^E_{kl}\, h_{lj} \\
&= \frac{1}{N}\sum_{k,l} (-1)^{\,(i*k)\,+\,(l*j)} \left((1-p)\delta_{k,l} + p\delta_{k\,\hat{}\,l, r_E}\right) \\
&= \frac{1}{N}\sum_{k} (-1)^{\,(i\,\hat{}\,j)*k}(1-p) + (-1)^{\,(i*k)+((k\,\hat{}\,r_E)*j)}\, p \\
&= \left((1-p) + (-1)^{r_E * j} p\right) \cdot \underbrace{\frac{1}{N}\sum_k (-1)^{(i\,\hat{}\,j)*k}}_{=\delta_{i,j}}
\end{aligned}
$$

The effect of an error $E$ can thus be described by a vector of length $N$. This can easily be generalized to a set of mutually exclusive error patterns. Given a distribution $P$ on a set $S = \{E;\ \sum_E P(E) = 1\}$ of mutually exclusive errors, the matrix elements in Hadamard basis are simply

$$(HT^S H)_{ij} = \delta_{i,j} \sum_{E \in S} P(E)(-1)^{r_E * i} \quad (2)$$

The set of all possible error patterns that can occur during one application of the circuit can be divided into sets of mutually exclusive errors:

Consider for example the errors due to a gate acting on $q$ qubits, with a probability distribution $P$ across all $q$-qubit errors $E$. $P$ can be expressed as the product of one or several independent distributions $p_i$.

$$P(E) = \sum_{\substack{\{E_1 \dots E_{n_p}\} s.t. \\ E = E_1 \cdot E_2 \cdot \dots E_{n_p}}} \prod_{i=1}^{n_p} p_i(E_i) \text{ with } \sum_E p_i(E) = 1 \ \forall i \quad (3)$$

The sum goes over all sets of $q$-qubit errors $\{E_i\}$ that add up to the error $E$. Note that the errors $E_i$ are *not* restricted to qubit $i$. Each distribution $p_i$ is specified by a set of mutually exclusive $q$-qubit errors. Consider for example a depolarizing channel that acts independently on each qubit. For any qubit, the probability of an $X$, $Y$, and $Z$ error is $p_{tot}/3$ for each. The error distribution is then the product of $q$ independent distributions

$$p_q(E) = \begin{cases} 0 & \text{if } \exists j \neq q \text{ s.t. } E|_j \neq \mathbb{I} \\ p_{tot}/3 & \text{if } E|_j = \mathbb{I} \ \forall j \neq q \text{ and } E|_q \neq \mathbb{I} \\ 1 - p_{tot} & \text{if } E = \mathbb{I} \end{cases}$$

where $\mathbb{I}$ denotes the identity.

As long as the individual error probabilities do not depend on the state of the system, the transition matrix describing the error propagation during the entire circuit is simply the product of the transition matrix for each set given by eq. (2). If errors caused by different gates are independent, calculating the total transition matrix $T$ in Hadamard basis then requires iterating over an array of length $N$ for each set of mutually exclusive errors of all gates during the circuit. This is absolutely doable as long as it is a one-time calculation. The calculated probabilities are stored in an xml- or text file and read in for all further simulations. The factor restricting our simulations with MLCLN is the memory requirement dictated by the storage space for this array of size $N$.

Now that we have the transition matrix it is in principle straightforward to see how the updating procedure would have to look like. Starting from a vector $v$ of length $N$, and assigning a probability one to the entry denoting the probability of having no error at all and zero to all other entries, the distribution after the first circuit application is then given by $H(HTH)Hv$. However, conditioned on the measured syndrome only $4^k 2^{n_a}$ entries remain while all other entries have to be set to zero. Resetting the ancilla qubits before each circuit application corresponds to subsequently setting the measured syndrome to the same value as the ideal syndrome for each EC-coset. Instead of working with the full vector of length $N$, it is therefore sufficient to update a smaller vector that contains the probability that a given combination of Pauli operator consistent with a certain ideal syndrome and a logical operation will correct the current state. We call such a combination the *representative* of a certain equivalence class of errors. Errors within one equivalence class differ only up to the application of members of the stabilizer group. Note that only the full transition matrix of size $N \times N$ is diagonal in Hadamard basis. This is not the case for the smaller matrix of size $4^k 2^{n_a} \times 4^k 2^{n_a}$, that is derived from the larger one and depends on the previous and the current value of the measured syndrome. Just like for the full transition matrix, every entry of the one-step probability vector is needed to generate this reduced transition matrix. Nonetheless, it is more efficient to work with the smaller matrix, since that requires only around $N$ multiplications and additions, whereas a fast Walsh-Hadamard transformation requires around $N \log_2 N$ additions each time, in addition to the $N$ multiplications for the application of the transition matrix in Hadamard basis.

On a phenomenological level, equivalence classes of errors are merely characterized by an ideal syndrome and a logical operator. The full transition matrix $T$ is then only of size $4^k 2^{n_a} \times 4^k 2^{n_a}$. It is independent on the measured syndrome values and diagonal in Hadamard basis. An update then consists of a multiplication with this modified transition matrix, followed by re-weighting each vector entry depending on the the difference between its ideal syndrome and the measured syndrome value. A more detailed description of this phenomenological approach can be found in Ref. 1. We would like to point out that a reasonable error correction for circuit level noise using this phenomenological maximum likelihood decoding relies on a fairly accurate (phenomenological) model for the circuit noise, based on which the reduced transition matrix as well as the syndrome error probabilities are calculated. Our initial approach of estimating individual qubit failure probabilities at the end of the circuit to define a phenomenological ML decoding failed for circuit level noise. This version is labeled as 'phenomenological ML' in Fig.3 and Fig.5. A more accurate noise model allows for a better performance and preserves the asymptotic decrease of the logical error rate, even if the model is of phenomenological nature. The most accurate phenomenological noise model is obtained by first calculating the one-step probability distribution for a full circuit level noise model, and then marginalizing separately over data qubit errors and syndrome qubit errors to get the modified transition matrix as well as the re-weighting based on the measured syndrome. Such an ML decoding based on an intricate phenomenological noise model is labeled 'approximated MLCLN' in Fig.3 and Fig.5.

*Minimum Weight Perfect Matching Decoding:* While for Toric codes defects indeed always arise in pairs, for surface codes errors along the boundary can result in a change of just one syndrome bit. The matching defect would be outside the scope of the code. We therefore need to allow a matching of each defect with its 'mirrored bit flip' that lays beyond the code boundary, which we will call its *spatial counterpart*. Similarly, due to imperfect syndrome extraction, defects need to be matched within a three-dimensional space-time cube of syndrome changes [2]. Since one half of a matching pair may

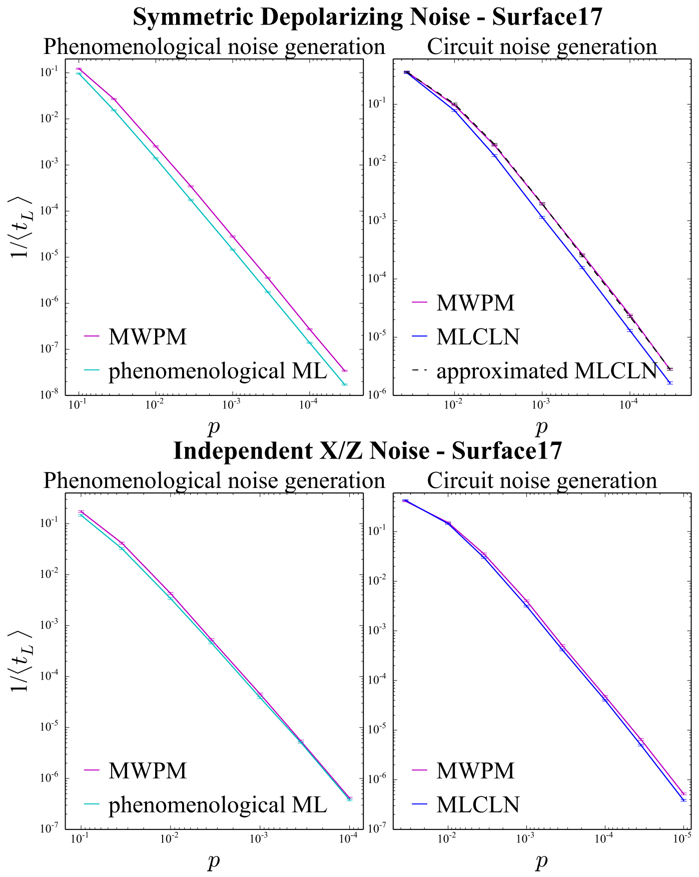


Figure 3. The left hand panel shows results for phenomenological noise, *i.e.* noise is generated according to individual qubit failure probabilities for both data and ancilla qubits. Within this framework, no circuit is applied. Correspondingly, a ML decoding based on this phenomenological noise model gives an optimal performance. For realistic, circuit level noise a decoder based on a phenomenological model - like *e.g.* the approximated version of MLCLN described in the main text - is suboptimal and performance strongly depends on the accuracy of the estimated data qubit failure rates at the end of the circuit.

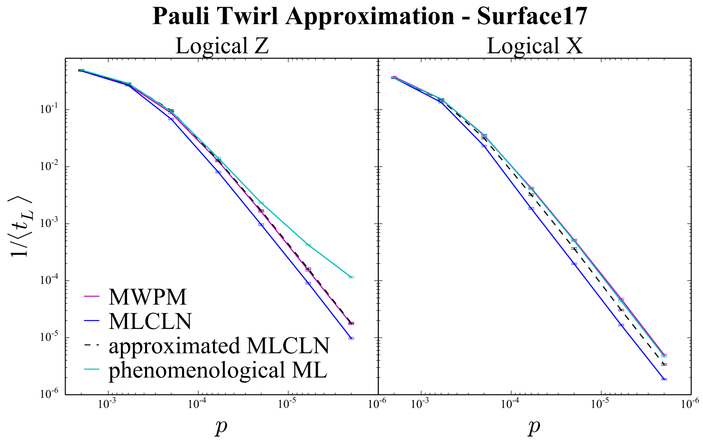


Figure 4. Pauli twirl approximation for amplitude damping noise during the syndrome extraction circuit as described in the main paper.

occur only after future rounds of syndrome extraction, each syndrome flip and its mirrored counterpart additionally need to be allowed to pair up with their counterpart mirrored along the time direction, which we will call their *time-like counterparts*. For a space-time cube containing $k$ detected changes of syndrome bits, we therefore find a perfect matching on a graph with $4k$ vertices. Note that only the $k_X$ ($k_Z$) vertices corresponding to the changes of $X$-type ($Z$-type) stabilizer measurements in each quadrant are fully connected, while pairings across spatial and time-like boundaries are only possible between detected flips and their individual counterparts. For any two flips that can be paired, so can their spatial counterpart, and for any possible pairing between a flip and its spatial counterpart, the corresponding pairing between the two time-like counterparts is possible as well. All pairings between counterparts - spatial or time-like - are free.

For a given space-time cube of measured bit flips, we use a Blossom algorithm to match pairs. Keeping track of both the latest matching as well as the corresponding correction for each pair throughout the algorithm allows to dynamically adapt the suggested correction based on new information. Such a 'moving decoding window' allows to handle an arbitrary length syndrome history, in spite of a limited memory. The maximum weight of a correctable data qubits error is given by code distance. It is reasonable to restrict the maximum weight along the time axis for correctable errors to the code distance as well. As soon as the last detected flip goes back longer than this maximum distance, it is reasonable to assume it will never be re-matched, and its paring along with the corresponding correction can therefore be discarded. This alone does not bound the required memory, since the occurring flips can be evenly spaced with a smaller time-like separation. We therefore define a *decoding depth*, that limits the number of pairs that are potentially broken up and re-matched in order to match a newly detected flip. The maximum length of the relevant history is then limited by two times the decoding depth multiplied by the maximum spatial pairing distance given by code size.

## IMPLEMENTATION AND SIMULATION

For both, maximum likelihood and MWPM decoding, corrections do not need to be applied. They can be kept in memory until the end of the algorithm and merely taken into account when reading out the result. This is mostly relevant for MLCLN, where actually applying a correction would require permuting all probabilities correspondingly and is therefore costly. For the evaluation of whether the decoder correctly predicts the logical state, we take the additional information obtained from a final measurement of all data qubits into account. This information would be available if it was indeed the end of an algorithm. Provided the predicted state is still correct, all further decoding does of course not rely on that information but solely on the measured syndrome values and the additional data qubit information of the final round.

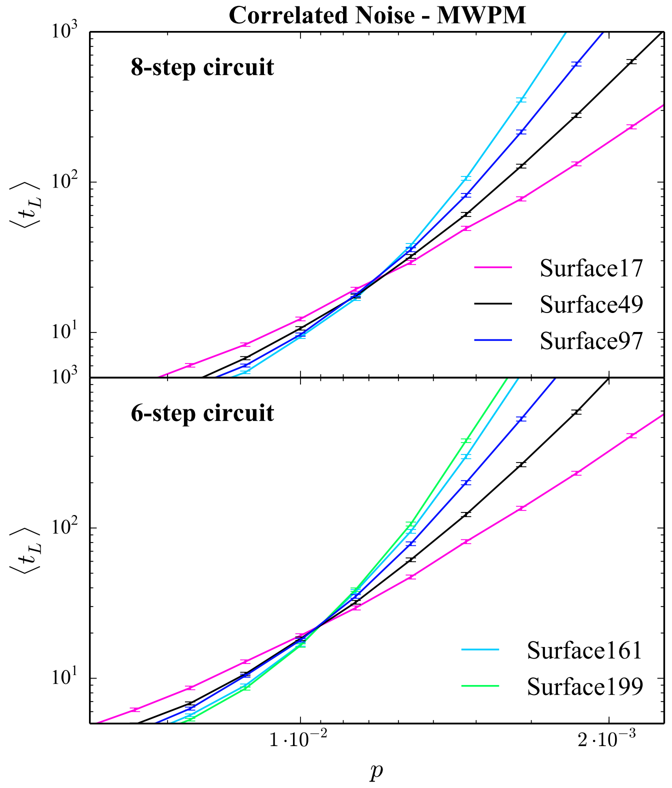


Figure 5. Comparison of the error threshold between a 6- and an 8-step syndrome measurement circuit for the noise model in Fig.1 of the main paper. The threshold probability for $X$ or $Y$ errors of 0.45% for the 8-step circuit still lays distinctly above the corresponding value of 0.28% for independent bit and phase flip noise on each qubit (Fig.2 in the main paper).

*Error Generation:* The stabilizer formalism allows to merely propagate the current error pattern through the applied circuit without having to keep track of the actual quantum state, as long as only Pauli errors occur. Instead of applying an error with a certain probability after the application of each gate in the circuit, we directly generate the time of the next failure for each gate. If a gate fails with probability $p \in (0,1)$, then the probability of a failure after exactly $k$ applications is $p(1-p)^{k-1}$ for $k \in \mathbb{N}$. Drawing $z$ from a uniform distribution in (0,1) and calculating

$$k = \left\lceil \frac{\log(1-z)}{\log(1-p)} \right\rceil \tag{4}$$

generates suitable values.

Error-free cycles give the decoder time to ascertain and improve its current knowledge about the system. However, once its state changes only insignificantly from round to round, there is no reason to simulate cycles during which no errors occur. Even more, we are only interested in the frequency of error combinations that lead to a decoding failure. Generating the times of the next error for each gate allows us to perform an importance sampling where we discard (some of the) irrelevant error combinations. We omit cycles for which we know that they will be processed correctly – i.e. cycles for which only correctable error combinations occur and both system and decoder are in equilibrium.

We consider the system to be equilibrated if the measured syndrome fully reflects the data qubit excitation pattern and there are no remaining excitations after applying the proposed correction. For MWPM the decoder equilibrium is reached if no syndrome changes were detected within the limited time covered by the decoding window explained above. In that case, the details about all previous pairings and their corrections have already been discarded, and only one total correction based on all previous rounds of decoding is kept in memory. To determine an equilibrium condition for an ML decoder, we test how much the error probability vector changes from one round to the next one. After initialization, we repeatedly update the decoder by passing it a measured syndrome value zero. After a few iterations, the maximal amount by which the vector changes from one update to another converges. For an ML decoder to be equilibrated we expect that any entry of the probability vector was changed by less than 1.1 times this value by the latest update.

To determine the most frequent error combinations that are correctable, prior to performing our simulations, we test the *recovery time* for all mutually exclusive errors in each independent error set of any gate during the simulated circuit. The recovery time denotes the time it takes for the decoder to correctly identify the data qubits error pattern and re-equilibrate. The tests are performed once for each simulation type – i.e. once for each combination of noise model, decoder, decoder configuration, and circuit. – and the found recovery times are stored in an xml-file. Any error combination during a simulation are nothing but a superposition of the tested error patterns. Knowing when each pattern occurs allows to omit simulating its effect, if system and decoder have been in equilibrium prior to its occurrence and the next error does not happen until after the system has recovered and the decoder has re-equilibrated.

In principle, also less likely sets of errors can be tested for their recoverability, but their rarity does not merit the exceeding computational effort of testing.

[1] S. Bravyi, Bulletin of the American Physical Society (2016).

[2] E. Dennis, A. Kitaev, A. Landahl, and J. Preskill, Journal of Mathematical Physics **43**, 4452 (2002).
